# Supplementary material for: Cancer Gene Profiling through Unsupervised Discovery
Source: arXiv:2102.07713 source file (2021-02-11)
Supplement: Supplementary file 2 [file Additional_File_1.pdf]

## **LP-Stability Gene Signature Biological Processes**

HSFX1: DNA binding transcription

C3P1: endopeptidase inhibitor activity

CCDC30: Coiled-Coil Domain

CNRIP1: cannabinoid receptor

CD53: regulation of cell development

SPRR4: UV-induced cornification

RIF1: DNA repair

COL1A2: collagen making

ZNF767: gene expression

CD3E: antigen recognition (linked to immunodeficiency)

MATR3: nucleic acid binding and nucleotide binding

NCAPH: Cell Cycle, Mitotic and Mitotic Prometaphase

ASH1L: transcriptional activators

ANKRD30A: DNA-binding transcription factor activity (related to breast cancer)

GNA15: among its related pathways are CREB Pathway and Integration of energy metabolism

GADD45GIP1: Among its related pathways are Mitochondrial translation and Organelle biogenesis and maintenance.

CD302: cell adhesion and migration

SFTA3: Among its related pathways are Surfactant metabolism and Diseases of metabolism.

C1orf159: Protein Coding gene

RPS8: Among its related pathways are Viral mRNA Translation and Activation of the mRNA upon binding of the cap-binding complex and eIFs, and subsequent binding to 43S.

ZEB2: Among its related pathways are MicroRNAs in cancer and TGF-beta Receptor Signaling

GSX1: sequence-specific DNA binding and proximal promoter DNA-binding transcription activator activity, RNA polymerase II-specific

ADNP: Vasoactive intestinal peptide is a neuroprotective factor that has a stimulatory effect on the growth of some tumor cells and an inhibitory effect on other

CLIP3: plays a role in T cell apoptosis by facilitating the association of tubulin and the lipid raft ganglioside GD3

YEATS2: Among its related pathways are Chromatin organization

ACBD4: Among its related pathways are Metabolism and Peroxisomal lipid metabolism

SNRPG: Among its related pathways are mRNA Splicing - Minor Pathway and Transport of the SLBP independent Mature mRNA
