# Supplementary material for: Cancer Gene Profiling through Unsupervised Discovery
Source: arXiv:2102.07713 source file (2021-02-11)
Supplement: Supplementary file 4 [file response.tex]

\documentclass[journal]{IEEEtran}
%%% Load packages
\usepackage{amsthm,amsmath}
%\RequirePackage{natbib}
%\RequirePackage[authoryear]{natbib}% uncomment this for author-year bibliography
%\RequirePackage{hyperref}
\usepackage[utf8]{inputenc} %unicode support
%\usepackage[applemac]{inputenc} %applemac support if unicode package fails
%\usepackage[latin1]{inputenc} %UNIX support if unicode package fails
\usepackage{multirow}
\usepackage{mwe}

\def\includegraphic{}
\def\includegraphics{}



%%% Put your definitions there:
\startlocaldefs
\endlocaldefs

\date{}
%%% Begin ...
\begin{document}
\title{Response to Reviewers}
\maketitle

\section{Reviewer 1}
REVIEWS

Reviewer: 1

Recommendation: Accept With No Changes

Comments:
This paper was very clear and easy to follow and makes a clear contribution to the field.

Additional Questions:
1.  Please explain how this manuscript advances this field of research and/or contributes something new to the literature.: This paper describes the application of the LP-Stability algorithm to cluster-based analysis of genes, and compares it with other standard clustering algorithms using various distance-based metrics. The paper uses TCGA data sets to compare results of the various algorithms. While this paper is an extension of a previously published conference article, it cites the conference article and clearly indicates how the two articles differ. It also contains substantially more technical information than the conference article.

2. Is the manuscript technically sound? Please explain your answer under Public Comments below.: Appears to be - but didn't check completely

1. Which category describes this manuscript?: Practice / Application / Case Study / Experience Report

2. How relevant is this manuscript to the readers of this periodical? Please explain your rating under Public Comments below.: Very Relevant

1. Are the title, abstract, and keywords appropriate? Please explain under Public Comments below.: Yes

2. Does the manuscript contain sufficient and appropriate references? Please explain under Public Comments below.: References are sufficient and appropriate

3. Does the introduction state the objectives of the manuscript in terms that encourage the reader to read on? Please explain your answer under Public Comments below.: Yes

4. How would you rate the organization of the manuscript? Is it focused? Is the length appropriate for the topic? Please explain under Public Comments below.: Satisfactory

5. Please rate the readability of the manuscript. Explain your rating under Public Comments below.: Easy to read

6. Should the supplemental material be included? (Click on the Supplementary Files icon to view files): Yes, as part of the digital library for this submission if accepted

7. If yes to 6, should it be accepted: As is

Please rate the manuscript. Please explain your answer.: Excellent


\section{Reviewer 2}

Recommendation: Revise and resubmit as “new”

Comments:
This manuscript presented a comparison of three methods, namely LP-stability based clustering, K-mean and CorEx on selected TCGA gene expression. The manuscript was organized like a computer science paper but the major contribution is the results and implication of the selected methods. The authors generated a substantial amount of results, some sounds interesting. I have the following major concerns to this manuscript:
\subsection{ Biological implications: Two types of successful application of sample-wise clustering analysis on cancer data include (i) disease stratification (such as the CMS classification of colon cancer) and (ii) like the immuno-landscape characterization cited in the manuscript. (i) focusing on subtype classification to optimize clinical relevance while (ii), with gene selection, focusing on characterization the range and possible classes of cancers with respect to a certain biological mechanism. However, in this manuscript, I cannot see significant biological implications from the results. Even the functions of the genes and clusters were discussed, how these clusters related to different disease property and clinical impact was not analyzed and discussed. I do not consider the current results can contribute significant insight to current understanding of cancer.}

The point raised here is indeed a key point.

We first want to highlight that the focus of this study, more than offering another analysis of clusters or even cancer signature, is to present a pipeline adaptable and general that enables to obtain such clusterings and signatures in any context and then analyzing them. Indeed, we feel that the normalization of clustering techniques and signatures comparisons is a very important yet not well studied aspect preventing any clear advance in the field. 

An additional point we want to clarify is that we aim here to focus on the discovery power of the signature we establish which justify the use of an unsupervised feature selection technique to define the signature. Besides, the point of this pipeline is to define a signature that is compact, redundancy-free and yet informative. The genes selected are so unbiased and not selected to answer a particular predictive task. They so might not well studied and so bringing a full biological analysis of their function would be very challenging. However, we brought a special attention to this very relevant comment in our revision. We so believe that this new submitted version is bringing sufficient proof of both the validity of the approach and of the informativeness of the signature proposed. 
To highlight the quality of the clustering method genes-wise, we so provide detailed results of enrichment score and Dunn's Index of the clusters with the proposed method, two referential methods and random clustering.
To justify the quality of the signature we performed a sample-wise clustering using as features our proposed signature, a referential signature from literature and random genes showing the superior ability of our signature to have a meaningful separation of samples into clusters has proven by the study of tumor types distribution and the analysis relying on SAM method.
We added in this revised version a supervised classification task. To show both that the signature while containing only $27$ genes still contain enough information and tissue-specific information in response to a comment of reviewer 2. We compared results to the ones using the referential signature from literature and random genes showing the highest informativeness of our signature.
We also provide in supplementary files the details of the genes involved and functions they are associated to. We  studied the enriched processes of the genes of the signature to prove the redundancy-freedom.On the kind advice of reviewer 2 we now report a summary of the GTEx portal analysis for each gene.

\subsection{ Gene signature selectioned: The authors offered clear introduction of the methods and implications except how the 27 genes were selected. As mentioned by the authors "The predictive power of the best signature per algorithm was further assessed by measuring its ability to separate in a completely unsupervised manner 10 different tumor types (Table II) through sample clustering.", if this is how the genes were selected, I highly doubt the genes are tissue specific genes, which should be tested by checking GETX data. I also concern the number of genes selected here are too small. How and what biological aspects can be well represented by the space spanned by the expression profile of the 27 selected genes need to be evaluated.}

We have taken care of this very relevant comment. In the revised version we now state at the beginning of section III-B:
"The best signature was selected for each clustering algorithm using the method detailed in section II-F on the clustering presenting the highest DI while having best ES."

\subsection{Rationality of the analysis and comparison: Three top factors that affect the TCGA gene expression data are (i) copy number varation in cancer cell, (ii) tissue components (cancer, immune and stromal cells) and (iii) tissue specific genes. Due to the selection of the ~30 genes can be biased to tissue specific genes or possible copy number varation, I concern the pathway enrichment analysis against PPI is too limited. Check the enrichment to MsigDB pathways of different biological meaning.}

This is a very relevant point. We are well aware of the limitations of the PPI Enrichment. However, as we want to establish here an automatic and unbiased pipeline of comparison of clusterings we wanted to avoid the use of enrichment in specific pathways. Indeed, so doing, we would have lost the generality of the comparison by considering only clusters that would be relevant according to some pre-defined functions or processes. Besides, we are interested in defining a new biological metric for clustering assessment which is a very relevant topic  though beyond the scope of this article.

Besides, anyone who would want to use our methodology for a different task could adapt both metrics we use at his convenience.

\subsection{I recommend the authors to test the methods on selected genes of certain functions, such as the immuno-response or metabolism or certain cancer hallmarkers and mine the landscape of the samples from different cancer types. Then the biological meaning of each cluster can be better annotated and the feature of the selected methods can be better seen.}

We take good note of this very relevant remark.
However, the aim of this study is to prove the validity of the methodology used and of the signature defined. We details in our response section II-A the different proofs we brought to these two points.

Additional Questions:
1.  Please explain how this manuscript advances this field of research and/or contributes something new to the literature.: Mining the performance of sample-wise clustering methods on cancer transcriptomics data.

2. Is the manuscript technically sound? Please explain your answer under Public Comments below.: Yes

1. Which category describes this manuscript?: Practice / Application / Case Study / Experience Report

2. How relevant is this manuscript to the readers of this periodical? Please explain your rating under Public Comments below.: Relevant

1. Are the title, abstract, and keywords appropriate? Please explain under Public Comments below.: No

2. Does the manuscript contain sufficient and appropriate references? Please explain under Public Comments below.: References are sufficient and appropriate

3. Does the introduction state the objectives of the manuscript in terms that encourage the reader to read on? Please explain your answer under Public Comments below.: Yes

4. How would you rate the organization of the manuscript? Is it focused? Is the length appropriate for the topic? Please explain under Public Comments below.: Satisfactory

5. Please rate the readability of the manuscript. Explain your rating under Public Comments below.: Readable - but requires some effort to understand

6. Should the supplemental material be included? (Click on the Supplementary Files icon to view files): Yes, as part of the digital library for this submission if accepted

7. If yes to 6, should it be accepted: After revisions.  Please include explanation under Public Comments below.

Please rate the manuscript. Please explain your answer.: Good

\section{Reviewer 3}
Recommendation: Revise and resubmit as “new”

Comments:
In this manuscript, the authors proposed a linear programming-based clustering method to identify the representative gene groups for molecular signature identification. Then based on the identified gene clusters, the tumor samples were stratified into different groups. The proposed framework was applied to large-scale TCGA datasets. The gene clustering algorithm was compared to K-means and CorEx algorithms and the performance was evaluated by Dunn's Index and the enrichment on the PPI network. The sample clustering results were evaluated by matching the clusters to different tumor types. The reviewer has the following concerns:

Major comments:
\subsection{ Biomarker identification is a very important step for drug discovery and targeted therapy to improve disease prognosis and diagnosis. Most proposed methods chose supervised feature selection methods to identify the molecular signatures that associate with clinical variables.  Why did the authors choose the unsupervised clustering method to identify signature genes? A better description is needed in the Introduction section.}

We acknowledge the importance to better justify the importance in our approach to rely on an unsupervised feature selection instead of a supervised one.

We were stating that "Unsupervised techniques such as clustering are very efficient for the study of large high-dimensional datasets and aim to discover unknown indiscernible structures and correlations".

In the revised version we so added in introduction "Besides, at the difference of supervised techniques meant to select features for a specific purpose, unsupervised clustering enables to discover unknown patterns, associations and correlations in the data."

\subsection{ The parameter 's' in equation S(q) on page 2 was not defined in the manuscript. In addition, how did the algorithm can automatically select the number of clusters?}

We corrected this overlook. this parameter 's' was the parameter minimize in the inferior bound of the formula. 

We clarified that this automatic determination of the number of clusters was performed thanks to the optimization performed on the function C of the primal problem which characterizes the assignation of a point to a given center. The number of clusters is so indirectly determined by this function as it is the number of centers that have a point assigned to them. Please refer to section II-B-1 for complete definition of the optimization problem.

\subsection{ Which PPI network was applied to calculate Enrichment Score? A reference is needed. It is better to do enrichment analysis on KEGG pathways and Gene Ontology terms to evaluate the biological relevance of the gene sets}

Thank you for this relevant comment, we added the reference of the PPI network used (from the String Consortium) for computing the enrichment in section II-D of the revised paper.

We gave details on the reasons of using PPI network for enrichment in response II-C.

\subsection{ It is better to use NMI and ARI to evaluate the sample clustering results in Figure 6. The higher the consistency with the tumor subtypes, the better the results.}

NMI and ARI are indeed very relevant metric for supervised clustering evaluation. However, they prevent any discovery of new patterns or associations between the samples which we were particularly focusing on by using an unsupervised technique as explained in response III-A. 

\subsection{ On page 9, it was mentioned that 'we look for genes that are expressed differently for the samples of one tumor type in a cluster compared to the other samples of the same tumor type'. It is still unclear how to select the significant genes from each gene cluster.}

Indeed, the details of the technique used for defining the significant genes (SAM method) are given in section II-D. Besides for clarity sake we added in the revised version reference to this method section.

Minor comments:
\subsection{ It is unclear to me how did the authors conclude that '10 times better' and '$35\%$ better' in the Abstract based on the experimental results.}

These comparisons are coming from the comparison of average scores in Dunn's Index (DI) and PPI Enrichment Score (ES) of our favored method (LP-Stability) and the referential clustering methods (K-Means and CorEx). 
We added a column with Average Di in the revised version for better clarity.
we can see that LP-Stability has in average a DI of 38.5\% while K-Means has only 1.2 and CorEx 0.6, so the score of LP-Stability is in fact more than 30 times higher, we so put this more precise number in the abstract.
Besides, we apologize for the typo but the improvement in average ES was in fact of 25\% and not 35\%, it has been corrected in revised version.

Besides, we do not take into account the results obtained withe the random clustering as in the abstract we compare to referential clustering techniques for which random clustering does not qualify.

\subsection{ Typos in the supplementary document. e.g., '?' in section III.}

Thank you for this comment, it has been addressed in the revised version.

Additional Questions:
1.  Please explain how this manuscript advances this field of research and/or contributes something new to the literature.: The authors proposed a linear programming based gene clustering algorithm to identify gene signatures that associate tumor types from large-scale gene expression data.

2. Is the manuscript technically sound? Please explain your answer under Public Comments below.: Partially

1. Which category describes this manuscript?: Research/Technology

2. How relevant is this manuscript to the readers of this periodical? Please explain your rating under Public Comments below.: Relevant

1. Are the title, abstract, and keywords appropriate? Please explain under Public Comments below.: Yes

2. Does the manuscript contain sufficient and appropriate references? Please explain under Public Comments below.: Important references are missing; more references are needed

3. Does the introduction state the objectives of the manuscript in terms that encourage the reader to read on? Please explain your answer under Public Comments below.: Could be improved

4. How would you rate the organization of the manuscript? Is it focused? Is the length appropriate for the topic? Please explain under Public Comments below.: Satisfactory

5. Please rate the readability of the manuscript. Explain your rating under Public Comments below.: Readable - but requires some effort to understand

6. Should the supplemental material be included? (Click on the Supplementary Files icon to view files): Yes, as part of the digital library for this submission if accepted

7. If yes to 6, should it be accepted: After revisions.  Please include explanation under Public Comments below.

Please rate the manuscript. Please explain your answer.: Fair

\end{document}
